# Supplementary material for: Revisiting Explicit Negation in Answer Set Programming
Source: arXiv:1907.11467 source file (2019-07-26)
Supplement: Supplementary file 1 [file appendix.tex]

%%%%%%%%%%%%%%%%%%%%%%%%%%%%%%%%%%%%%%%%
\newpage
\section*{Appendix A. Proofs}

\begin{proofof}{Proposition~\ref{prop:total_model_reduct}}
We use structural induction on $F$. Notice that, when $F=\neg G$ and $T$ is a consistent set of literals, we have both:
\[
\begin{array}{c@{\hspace{40pt}}c}
\begin{array}{rcl}
T \models \neg G	& \mbox{iff} &  T \not \models G \\
&  \mbox{iff} &   \left(\neg G\right)^T= \top \\
&  \mbox{iff} &  T \models \left(\neg G\right)^T
\end{array}
&
\begin{array}{rcl}
T \falsif \neg G	& \mbox{iff} & T   \models G \\
&  \mbox{iff} &  \left(\neg G\right)^T=\bot \\
&  \mbox{iff} &  T \falsif \left(\neg G\right)^T
\end{array}
\end{array}
\]
\end{proofof}

%%%%%%%%%%%%%%%%%%%%%%%%%%%%%%%%%%%%%%%%
\begin{proofof}{Theorem~\ref{th:httaut}}
Let $\At$ be the set of atoms occurring in $\varphi$ or in $\alpha$.
Suppose $\varphi$ is HT valid.
Without loss of generality, we can assume that $\alpha$ belongs to signature $\At\setminus\{p\}$ because, being $\varphi$ HT-valid, we can always replace any atom $p$ by a fresh one $p'$ and restate the theorem for the latter.
Now, suppose $\varphi[\alpha/p]$ is not $\X5$ valid.
Then, there is some $\X5$ interpretation $M=\tuple{H,T}$ for signature $\At\setminus\{p\}$ such that $M \not\models \varphi[\alpha/p]$ in $\X5$.
But then, we can construct an HT interpretation $\tuple{H',T'}$ for signature $\At$ that assigns atom $p$ the same behaviour as $\alpha$.
Formally: 
\[
H'=\left\{ \begin{array}{lcl} H & \mbox{ if } \tuple{H,T} \not \models \alpha \\
H \cup \{p\} &\mbox{ if } \tuple{H,T} \models \alpha
\end{array} \right. \hspace{1cm} 
T'=\left\{ \begin{array}{lcl} T  & \mbox{ if } \tuple{T,T} \not \models \alpha \\
T \cup \{p\} &\mbox{ if } \tuple{T,T} \models \alpha
\end{array} \right.
\]
for $p$ an atom and $\alpha$ a formula. 
It can be easily proved by induction on $\varphi$ that:
\begin{center}
$\tuple{H,T} \models \varphi[\alpha/p]$ iff $\tuple{H',T'} \models \varphi$
\end{center}
Since we had $\tuple{H,T} \not\models \varphi[\alpha/p]$, then $\tuple{H',T'}\not\models \varphi$, which contradicts that $\varphi$ is HT valid.
\end{proofof}

%%%%%%%%%%%%%%%%%%%%%%%%%%%%%%%%%%%%%%%%
\begin{proofof}{Lemma~\ref{lem:satisfaction_total_models}}
Use induction on $F$ and definitions of $T \models F$ from Section~\ref{sec:nested} and $\tuple{T,T} \models F$ from Definition~\ref{def:satfals}.
\end{proofof}

%%%%%%%%%%%%%%%%%%%%%%%%%%%%%%%%%%%%%%%%
\begin{proofof}{Theorem~\ref{th:persistence}}
Take $M=\tuple{H,T}$ an $\X5$-interpretation and $\varphi$ a formula. We are going to prove both (i) and (ii) by structural induction on $\varphi$. 
\begin{itemize}
\item If $\varphi=p$ and $\tuple{H,T} \models p$, then $p \in H \subseteq T$ which implies $\tuple{T,T}  \models p$. In case $\tuple{H,T} \falsif p$, we have that $\sneg p \in H \subseteq T$ and $\tuple{T,T}  \falsif p$.
\item If $\varphi= \alpha \wedge \beta$ and $\tuple{H,T} \models \varphi$, then both $\tuple{H,T} \models \alpha$ and $\tuple{H,T} \models \beta$. By induction, $\tuple{T,T} \models \alpha$ and $\tuple{T,T} \models \beta$ or, equivalently $\tuple{T,T} \models \alpha \wedge \beta$. Now suppose that $\tuple{H,T} \falsif \varphi$, then  $\tuple{H,T} \falsif \alpha$ or $\tuple{H,T} \falsif \beta$. By induction, $\tuple{T,T} \falsif \alpha$ or $\tuple{T,T} \falsif \beta$  which means that $\tuple{T,T} \falsif \alpha \wedge \beta$.
\item If $\varphi= \alpha \vee \beta$, the proof is similar to the previous case.
\item If $\varphi = \sneg \alpha$ and $\tuple{H,T} \models \varphi$, then $\tuple{H,T} \falsif \alpha$ and, by induction $\tuple{T,T} \falsif \alpha$ or $\tuple{T,T} \models \varphi$. If $\tuple{H,T} \falsif \varphi$, then $\tuple{H,T} \models \alpha$ and, by induction $\tuple{T,T} \models \alpha$ or $\tuple{T,T} \falsif \varphi$. 
\item If $\varphi = \alpha \to \beta$ and $\tuple{H,T} \models \varphi$, then [$\tuple{H,T} \not\models   \alpha \mbox{ or } \tuple{H,T} \models \beta$] and [$\tuple{T,T} \not\models   \alpha \mbox{ or } \tuple{T,T} \models \beta$] which implies that $\tuple{T,T} \models \varphi$ by definition. Now suppose that $\tuple{H,T} \falsif \varphi$. Then, $\tuple{T,T} \models \alpha$ and $\tuple{H,T} \falsif \beta$. By induction $\tuple{T,T} \falsif \beta$, so $\tuple{T,T} \falsif \varphi$.
\end{itemize}
\end{proofof}

%%%%%%%%%%%%%%%%%%%%%%%%%%%%%%%%%%%%%%%%
\begin{proofof}{Proposition~\ref{prop:default_negation}}
By applying Theorem~\ref{th:persistence}, we know that $\tuple{T,T} \not \models \varphi$ implies $\tuple{H,T} \not \models \varphi$. This proves that $\tuple{H,T} \models \neg \varphi : \varphi \to \bot$ iff $\tuple{T,T} \not \models \varphi$. On the other hand, $\tuple{H,T} \falsif \neg \varphi$ iff $\tuple{T,T} \models \varphi$ and $\tuple{H,T} \falsif \bot$ or, equivalently,  $\tuple{T,T} \models \varphi$.
\end{proofof}

%%%%%%%%%%%%%%%%%%%%%%%%%%%%%%%%%%%%%%%%
\begin{proofof}{Lemma~\ref{lem:aux_reduct}}
%\comment{To be completed}
We proceed by structural induction on $F$.
If $F=p$, take into account that $p^T=p$. First of all, $\tuple{H,T} \models p$ iff $p \in H$. On the other hand, $\tuple{H,T} \falsif p$ iff $H \models \sneg p$, or equivalently  $H \falsif p$ \\
Now suppose that $F=F_1 \wedge F_2$. Then, it follows:
\begin{align*}
\tuple{H,T} \models F	&\ \ \mbox{ iff } \ \ \tuple{H,T} \models F_1 \mbox{ and } \tuple{H,T} \models F_2
\\
	&\ \ \mbox{ iff } H \models (F_1)^T \mbox{ and }  H \models (F_2)^T
\\
	&\ \ \mbox{ iff } H \models (F_1)^T \wedge (F_2)^T
\\
		&\ \ \mbox{ iff } H \models (F_1 \wedge F_2)^T
\end{align*}
Also:
\begin{align*}
\tuple{H,T} \falsif F	&\ \ \mbox{ iff } \ \ \tuple{H,T} \falsif F_1 \mbox{ or } \tuple{H,T} \falsif F_2
\\
	&\ \ \mbox{ iff } H \falsif (F_1)^T \mbox{ or }  H \falsif (F_2)^T
\\
	&\ \ \mbox{ iff } H \falsif (F_1)^T \wedge (F_2)^T
\\
		&\ \ \mbox{ iff } H \falsif (F_1 \wedge F_2)^T
\end{align*}

\noindent The proof of the case $F= F_1 \vee F_2$ is similar.\\
We can also use Lemma~\ref{lem:satisfaction_total_models} and Proposition~\ref{prop:default_negation} to prove that
\begin{align*}
\tuple{H,T} \models \neg F	& \mbox{ iff }  \tuple{T,T} \not \models F \\
	& \mbox{ iff }  T \not \models F \\
&  \mbox{ iff }  \left(\neg F\right)^T= \top \\
&  \mbox{ iff }  H \models \left(\neg F\right)^T
\end{align*}
 and
\begin{align*}
\tuple{H,T} \falsif \neg F	& \mbox{ iff }  \tuple{T,T}   \models F \\
& \mbox{ iff }  T   \models F \\
&  \mbox{ iff }  \left(\neg F\right)^T=\bot \\
&  \mbox{ iff }  H \falsif \left(\neg F\right)^T
\end{align*}
\\
Finally:
\begin{align*}
\tuple{H,T} \models \sneg F	&\ \ \mbox{ iff } \ \ \tuple{H,T} \falsif F
\\
	&\ \ \mbox{ iff } H \falsif F^T 
\\
	&\ \ \mbox{ iff } H \models \sneg\left(F^T\right)
\\
		&\ \ \mbox{ iff } H \models \left(\sneg F\right)^T
\end{align*}
 and
\begin{align*}
\tuple{H,T} \falsif \sneg F	&\ \ \mbox{ iff } \ \ \tuple{H,T} \models F
\\
	&\ \ \mbox{ iff } H \models F^T
\\
	&\ \ \mbox{ iff } H \falsif \sneg(F^T)
\\
		&\ \ \mbox{ iff } H \falsif \left(\sneg F \right)^T
\end{align*}
\end{proofof}

%%%%%%%%%%%%%%%%%%%%%%%%%%%%%%%%%%%%%%%%
\begin{proofof}{Corollary~\ref{cor:equivalence_for_total_model}}
Notice that, when $F$ is any nested expression, we have that:
\begin{center}
$\tuple{T,T} \models F$ iff $T \models F$ iff  $T \models F^T$
\end{center}
by applying Lemma~\ref{lem:satisfaction_total_models} and Proposition~\ref{prop:total_model_reduct}.
\end{proofof}

%%%%%%%%%%%%%%%%%%%%%%%%%%%%%%%%%%%%%%%%
\begin{proofof}{Proposition~\ref{prop:htreduct}}
Take $r:F \to G$ any rule of $\Pi$. First of all, suppose that $\tuple{H,T} \models r$. By persistence, we know that $\tuple{T,T} \models r$, so $T$ is a model of $r$ because of Corollary~\ref{cor:equivalence_for_total_model}. Moreover:  
\[
\begin{array}{l}
\tuple{H,T} \not\models   F \mbox{ or } \tuple{H,T} \models G, \mbox{ and } \\
 \tuple{T,T} \not\models   F \mbox{ or } \tuple{T,T} \models G
\end{array}
\]
\noindent By applying Lemma~\ref{lem:aux_reduct}, we can say that $H \not\models   F^T$ or $H \models G^T$, so $H \models F^T \to G^T$. \\
For the other direction, if $H$ is a model of $r^T:F^T \to G^T$ and $T$ is a model of $r$, we have that $H \not \models F^T$ or $H \models G^T$. Using Lemma~\ref{lem:aux_reduct}, we can say that $\tuple{H,T} \not \models F$ or $\tuple{H,T} \models G$. The fact that $T$ is a model of $r$ allow us to conclude that $\tuple{H,T} \models r$.
\end{proofof}

%%%%%%%%%%%%%%%%%%%%%%%%%%%%%%%%%%%%%%%%
\begin{proofof}{Theorem~\ref{th:answersets}}
Suppose that $T$ is an answer set of a program $\Pi$. Then $\tuple{T,T} \models \Pi$ by Corollary~\ref{cor:equivalence_for_total_model}. If $H \subseteq T$ is such that $\tuple{H,T} \models \Pi$, we know by Proposition~\ref{prop:htreduct} that $H \models \Pi^T$. By minimality of $T$, we conclude that $H=T$. The proof of the other direction is similar.
\end{proofof}

%%%%%%%%%%%%%%%%%%%%%%%%%%%%%%%%%%%%%%%%

\review{
\begin{proofof}{Theorem~\ref{th:Ferraris_reduct}}
For proving (i), if $T \not\models \varphi$ then both $\tuple{H,T} \not\models \varphi$ (by persistence) and $\varphi^T_+=\bot$ (by definition) and the result trivially follows. Similarly, for (ii), when $T \not\falsif \varphi$ both $\tuple{H,T} \not\falsif \varphi$ (by persistence) and $\varphi^T_-=\top$. So, we assume $T\models \varphi$ for (i) and $T \falsif \varphi$ for (ii).
We are going to prove both (i) and (ii) by structural induction on $\varphi$. 

\begin{itemize}
\item If $\varphi=p$ and $T\models p$, we know that $p\in H$ iff $\tuple{H,T} \models p$ iff $H \models p=p^T$. In case that $T\falsif p$, we have that $\tuple{H,T} \falsif p$ iff $\sneg p \in H$ iff $H\falsif p=p^T$.

\item Suppose that $\varphi= \alpha \wedge \beta$ and $T\models \varphi$. Then both $T \models \alpha$ and $T \models \beta$. 
Notice that $\tuple{H,T} \models \varphi$ iff $\tuple{H,T} \models \alpha$ and $\tuple{H,T} \models \beta$. By induction, this is equivalent to $H \models \alpha^T_+$ and $H \models \beta^T_+$, that is, $H\models \varphi^T_+ = \alpha^T_+ \wedge \beta^T_+$.
On the other hand, $\tuple{H,T} \falsif \varphi$ iff $\tuple{H,T} \falsif \alpha$ or $\tuple{H,T} \falsif \beta$. By induction, this is equivalent to $H \falsif \alpha^T_-$ or $H \falsif \beta^T_-$, that is, $H\falsif \varphi^T_- = \alpha^T_- \wedge \beta^T_-$.

\item If $\varphi= \alpha \vee \beta$, the proof is similar to the previous case.

\item If $\varphi = \alpha \to \beta$ and $T \models \varphi$. First of all, suppose that $T\models \alpha$ and $H\models \varphi^T_+=\neg (\alpha^T_+) \vee \beta^T_+$. We want to prove that $\tuple{H,T}\models \varphi$. We can consider that $\tuple{H,T}\models \alpha$, which is the same, by induction, that $H\models \alpha^T_+$. This implies that $H\models \beta^T_+$. Finally, applying induction and taking into account that $T\models \beta$, we can conclude that $\tuple{H,T}\models \beta$. For the other direction, we proceed in a similar way. 

In the case that $T\not\models\alpha$, we have that $\alpha^T_+=\bot$. So, for any, $H\subseteq T$, it holds that $\tuple{H,T}\not\models\alpha$ and $H\models \neg(\alpha^T_+)$.

On the other hand, when $T\falsif \varphi$, we know that $T\models \alpha$ and $T\falsif\beta$, and we have to show that $H\falsif\varphi^T_-=\beta^T_-$ iff $\tuple{H,T}\falsif\varphi$. This latter is equivalent to $\tuple{H,T}\falsif\beta$ or, by induction, to $H\falsif\beta^T_-$.

\item When $\varphi = \neg \alpha$ and $T \models \varphi$ then $T\not\models\alpha$. This implies two things: first, by Proposition~\ref{prop:default_negation} we conclude $\tuple{H,T}\models \neg \alpha =\varphi$ and second, by persistence, $\tuple{H,T} \not\models \alpha$. By induction on the latter, $H \not\models \alpha^T_+$ and thus $H \models \neg (\alpha^T_+) = \varphi^T_+$.
For proving (ii), if $T \falsif \varphi$ then $T \models \alpha$. By Proposition~\ref{prop:default_negation}, this implies $\tuple{H,T} \falsif \neg \alpha =\varphi$ but we also have $\varphi^T_-=\bot$ and $H \falsif \bot$ trivially.

\item When $\varphi = \sneg \alpha$ and $T \models \varphi$, we know that $T\falsif\alpha$. Then, $\tuple{H,T}\models\varphi$ iff $\tuple{H,T}\falsif\alpha$. Using induction, we can say that this is equivalent to $H\falsif \alpha^T_-$ which coincides, by definition, with $H\models \sneg(\alpha^T_-)=\varphi^T_+$. In the case that $T\falsif\varphi$, we have that $T\models\alpha$. So by induction, we can assure that $\tuple{H,T}\models\alpha$ iff $H\models\alpha^T_+$. Using that  $\tuple{H,T}\models\alpha$ iff  $\tuple{H,T}\falsif\sneg\alpha$ and $H\models \alpha^T_+$ iff $H\falsif\sneg(\alpha^T_+)$, we can conclude the result.
\end{itemize}
\end{proofof}}{\ref{rev1.1}}
%%%%%%%%%%%%%%%%%%%%%%%%%%%

%%%%%%%%%%%%%%%%%%%%%%%%%%%%%%%%%%%%%%%%
\begin{proofof}{Theorem~\ref{th:corresp}}
\begin{itemize}
\item When $\varphi =p$, we know that $\tuple{H,T} \models p$ iff $p \in H$ or $M(p)=2$. Moreover $\tuple{T,T} \models p$ iff $M(p)=1$ or $M(p)=2$, that is, $M(p) >0$. On the other hand, $\tuple{H,T} \falsif p$ iff $\sneg p \in H$ iff $M(p)=-2$. Finally, $\tuple{T,T} \falsif p$ iff $\sneg p \in T$ iff $M(p)=-1$ or $M(p)=-2$, that is $M(p)<0$.
\item Suppose that $\varphi=\varphi_1 \wedge \varphi_2$. It follows that: 
\[
\begin{array}{lcl}
\tuple{H,T} \models \varphi_1 \wedge \varphi_2	& \mbox{ iff } & \tuple{H,T} \models \varphi_1  \mbox{ and }  \tuple{H,T} \models \varphi_2
\\
	&\mbox{ iff } & M(\varphi_1)=2  \mbox{ and }   M(\varphi_2)=2
\\
	& \mbox{ iff } & min(M(\varphi_1), M(\varphi_2))=2
\\
		& \mbox{ iff } & M(\varphi_1 \wedge \varphi_2)=2
\end{array}
\]
 and

\[
\begin{array}{lcl}
\tuple{H,T} \falsif \varphi_1 \wedge \varphi_2	&  \mbox{ iff } &  \tuple{H,T} \falsif \varphi_1  \mbox{ or } \tuple{H,T} \falsif \varphi_2
\\
	& \mbox{ iff } & M(\varphi_1)=-2  \mbox{ or }   M(\varphi_2)=-2
\\
	& \mbox{ iff } & min(M(\varphi_1), M(\varphi_2))=-2
\\
		& \mbox{ iff } & M(\varphi_1 \wedge \varphi_2)=-2
\end{array}
\]

We can also prove that:
\[
\begin{array}{lcl}
\tuple{T,T} \models \varphi_1 \wedge \varphi_2	&   \mbox{ iff } &  \tuple{T,T} \models \varphi_1  \mbox{ and }  \tuple{T,T} \models \varphi_2
\\
	&  \mbox{ iff } & M(\varphi_1)>0  \mbox{ and }   M(\varphi_2)>0
\\
	&  \mbox{ iff } & min(M(\varphi_1), M(\varphi_2))>0
\\
		&  \mbox{ iff } & M(\varphi_1 \wedge \varphi_2)>0
	\end{array}
\]

and
 \[
\begin{array}{lcl}
\tuple{T,T} \falsif \varphi_1 \wedge \varphi_2	&  \mbox{ iff } &   \tuple{T,T} \falsif \varphi_1   \mbox{ or }   \tuple{T,T} \falsif \varphi_2
\\
	& \mbox{ iff } & M(\varphi_1)<0   \mbox{ or }   M(\varphi_2)<0
\\
	& \mbox{ iff } & min(M(\varphi_1), M(\varphi_2))<0
\\
		& \mbox{ iff } & M(\varphi_1 \wedge \varphi_2)<0
	\end{array}
\]

\item The proof of the case $\varphi=\varphi_1 \vee \varphi_2$ is similar.
\item Suppose that $\varphi=\varphi_1 \to \varphi_2$. It follows that: 
\[
\begin{array}{lclcl}
\tuple{H,T} \models \varphi_1 \to \varphi_2	& \mbox{ iff } & \left\{\begin{array}{c}\tuple{H,T} \not \models \varphi_1  \mbox{ or }  \tuple{H,T} \models \varphi_2 \\
\mbox{ and } \\ \tuple{T,T} \not \models \varphi_1  \mbox{ or }  \tuple{T,T} \models \varphi_2 \end{array}
\right. & \mbox{ iff } & \left\{\begin{array}{c} M(\varphi_1)\neq 2  \mbox{ or }  M( \varphi_2)=2 \\
\mbox{ and } \\ M(\varphi_1) \leq 0  \mbox{ or }  M(\varphi_2)>0 \end{array} \right. \\
& & & & \\
& \mbox{ iff }  & \left\{\begin{array}{c} M(\varphi_1)\leq 0  \\
\mbox{ or } \\ M(\varphi_1) \neq 2  \mbox{ and }  M(\varphi_2)>0 \\
\mbox{ or } \\
M(\varphi_2)=2
\end{array} \right.& \mbox{ iff }  & M(\varphi_1 \to \varphi_2)=2
\end{array}
\]
 and

\[
\begin{array}{lcl}
\tuple{H,T} \falsif \varphi_1 \to \varphi_2	&  \mbox{ iff } &  \tuple{T,T} \models \varphi_1  \mbox{ and } \tuple{H,T} \falsif \varphi_2
\\
	& \mbox{ iff } & M(\varphi_1)>0 \mbox{ and }   M(\varphi_2)=-2
\\
		& \mbox{ iff } & M(\varphi_1 \to \varphi_2)=-2
\end{array}
\]

We can also show that:
\[
\begin{array}{lcl}
\tuple{T,T} \models \varphi_1 \to \varphi_2	&   \mbox{ iff } &  \tuple{T,T} \not \models \varphi_1  \mbox{ or }  \tuple{T,T} \models \varphi_2
\\
	&  \mbox{ iff } & M(\varphi_1)\leq 0  \mbox{ and }   M(\varphi_2)>0
\\
	&  \mbox{ iff } & M(\varphi_1 \to \varphi_2)>0
	\end{array}
\]

and
 \[
\begin{array}{lcl}
\tuple{T,T} \falsif \varphi_1 \to \varphi_2	&  \mbox{ iff } &   \tuple{T,T} \models \varphi_1   \mbox{ and }   \tuple{T,T} \falsif \varphi_2
\\
	& \mbox{ iff } & M(\varphi_1)>0   \mbox{ and }   M(\varphi_2)<0
\\
	& \mbox{ iff } & M(\varphi_1 \to \varphi_2)<0
	\end{array}
\]
\item Since $\tuple{H,T} \models \sneg \varphi$ (resp. $\tuple{H,T} \falsif \sneg \varphi$) iff $\tuple{H,T} \falsif \varphi$ (resp. $\tuple{H,T} \models \varphi$) and the fact that $M(\sneg \varphi)=-M(\varphi)$ complete the proof for $\sneg \varphi$.
\end{itemize}
\end{proofof}

%%%%%%%%%%%%%%%%%%%%%%%%%%%%%%%%%%%%%%%%
\begin{proofof}{Proposition~\ref{prop:leq}}
For the left to right direction, if $M \leq M'$, we have  $M=\tuple{H,T}$ and $M'=\tuple{H',T}$ with $H \subseteq H'$. Then, case 1 holds since, for any atom $p$, $M(p)=0$ iff $\{p,\sneg p\} \cap T = \emptyset$ iff $M'(p)=0$. 
For case 2, $M(p) \in \{1,2\}$.
Take $M(p)=2$, then $p \in H \subseteq H'$ and $M'(p)=2$. If, instead, $M(p)=1$, we conclude $p \in T \setminus H$ and, as $p \in T$, it means $M'(p) \geq 1=M(p)$. Case 3 with $M(p) <0$ is proved in an analogous way. For the right to left direction, suppose cases 1, 2 and 3 hold and let  $M=\tuple{H,T}$ and $M'=\tuple{H',T'}$.
We prove first that $T \subseteq T'$.
For any $p \in T$ we get $0< M(p) \leq M'(p)$ which means $p \in T'$.
Analogously, when $\sneg p \in T$ we obtain $0 > M(p) \geq M'(p)$ that implies $\sneg p \in T'$.
Direction $T' \subseteq T$ is analogous, and we conclude $T=T'$.
We prove now that $H \subseteq H'$.
Any $p \in H$ satisfies $M(p)=2$, and so, $M'(p) \geq M(p) = 2$ which implies that $M'(p)=2$, that is $p \in H'$. 
Similarly, for any $\sneg p \in H$ we have $M(p)=-2$, so $M'(p) \leq M(p)= -2$ which implies that $M'(p)=-2$, that is $\sneg p \in H'$.
\end{proofof}

%%%%%%%%%%%%%%%%%%%%%%%%%%%%%%%%%%%%%%%%
\begin{proofof}{Proposition~\ref{prop:replace}}
We just prove the left to right direction (the other one is symmetric).
Suppose that $M \models \Gamma \cup \{\alpha\}$.
Since $M \models \alpha$, we conclude $M(\alpha)=2$.
On the other hand, as $\alpha \leftrightarrow \beta$ is a tautology, $M(\alpha \leftrightarrow \beta)=2$ and, with $M(\alpha)=2$ the only possibility is $M(\beta)=2$, that is, $M \models \beta$.
Therefore, we immediately get $M \models \Gamma \cup \{\beta\}$.
\end{proofof}

%%%%%%%%%%%%%%%%%%%%%%%%%%%%%%%%%%%%%%%%
\begin{proofof}{Theorem~\ref{th:subst}}
As we saw in Figure~\ref{fig:tables}, $M(\alpha \Leftrightarrow \beta)=2$ iff $M(\alpha)=M(\beta)$.
Since $\models \alpha \Leftrightarrow \beta$, this means that $\alpha$ and $\beta$ have the same valuation for any $M$.
Since valuation of formulas is compositional, $M(\varphi[\alpha/p])=M(\varphi[\beta/p])$ and so $M(\varphi[\alpha/p] \Leftrightarrow \varphi[\beta/p])=2$ for any $M$.
\end{proofof}

%%%%%%%%%%%%%%%%%%%%%%%%%%%%%%%%%%%%%%%%
\begin{proofof}{Theorem~\ref{th:replace}}
We can suppose that $p \in \At(\varphi)$ because, otherwise, $\varphi[\alpha/p]=\varphi[\beta/p]=\varphi$. Since $p$ does not occur in the scope of explicit negation, we can also suppose that $\varphi \neq \sneg \psi$. The proof follows by structural induction on $\varphi$. We are going to suppose that $\tuple{H,T} \models \psi[\alpha/p]$ iff $\tuple{H,T} \models \psi[\beta/p]$ for any subformula $\psi$ of $\varphi$ and any $\X5$-interpretation $\tuple{H,T}$.
\begin{itemize}
\item If $\varphi=p$, then $\varphi[\alpha/p]=\alpha$ and $\varphi[\beta/p]=\beta$ and we have $\models \alpha \leftrightarrow \beta$ .
\item If $\varphi= \varphi_1 \wedge  \varphi_2$ and $\tuple{H,T} \models \varphi[\alpha/p]$, then both $\tuple{H,T} \models \varphi_1[\alpha/p]$ and $\tuple{H,T} \models \varphi_2[\alpha/p]$. By induction, $\tuple{H,T} \models \varphi_i[\beta/p]$, for $i=1,2$, so $\tuple{H,T} \models \varphi[\beta/p]$.
\item If $\varphi=\varphi_1 \vee  \varphi_2$, the proof is similar to the previous case.
\item If $\varphi = \varphi_1 \to  \varphi_2$ and $\tuple{H,T} \models \varphi[\alpha/p]$, then \big[$\tuple{H,T} \not \models \varphi_1[\alpha/p] \mbox{ or } \tuple{H,T} \models  \varphi_2[\alpha/p]$\big] and \big[$\tuple{T,T} \not\models  \varphi_1[\alpha/p] \mbox{ or } \tuple{T,T} \models  \varphi_2[\alpha/p]$\big] which implies, by induction, that \big[$\tuple{H,T} \not \models \varphi_1[\beta/p]$ or $\tuple{H,T} \models  \varphi_2[\beta/p]$\big] and \big[$\tuple{T,T} \not\models  \varphi_1[\beta/p]$ or $\tuple{T,T} \models  \varphi_2[\beta/p]$\big]. This means that $\tuple{H,T} \models \varphi[\beta/p]$.
\end{itemize}
\end{proofof}

\begin{proofof}{Lemma~\ref{lem:strong.equivalence.aux}}
First note that $\tuple{H,T} \models \alpha$
implies that $\tuple{H \cap \At(\alpha), T \cap \At(\alpha)} \models \alpha$
and, since $\alpha$ is finite we have that $\At(\alpha)$ is finite.
Hence, we assume without loss of generality that $\tuple{H,T}$ is finite.
Let $M = \tuple{H,T}$ and $M^t = \tuple{T,T}$.
Note that $M \models \alpha$ implies $M^t \models \alpha$ 
(Theorem~\ref{th:persistence}).
In case that $M^t \not\models \beta$,
let $\Delta = T$.
Then, $M^t$ is an equilibrium model of
$\Delta \cup \set{\alpha}$ but not of $\Delta \cup \set{\beta}$.
Otherwise, $H \neq T$ and we define:
$$\Delta = H \cup \setm{l_1 \to l_2}{l_1,l_2 \in T \setminus H}.$$
We can prove that $M$ is an equilibrium model of $\Delta \cup \set{\beta}$ but not of $\Delta \cup \set{\alpha}$. In fact, if $M'=\tuple{H',T}$ is a model of $\Delta \cup \set{\beta}$, then $H \subseteq H'$ but $H \neq H'$ because $\tuple{H,T} \not \models \beta$. If $H' \neq T$, we can find $l_1 \in H' \setminus H$ and $l_2 \in T \setminus H'$. But, then $l_1 \to l_2 \in \Delta$ and $\tuple{H',T} \not \models l_1 \to l_2$. This proves that $M$ is an equilibrium model of $\Delta \cup \set{\beta}$. The fact that $\tuple{H,T} \models \Delta \cup \set{\alpha}$ and $H \neq T$ implies that $M$ is not an equilibrium model of $\Delta \cup \set{\alpha}$.
\end{proofof}

%%%%%%%%%%%%%%%%%%%%%%%%%%%%%%%%%%%%%%%%
\begin{proofof}{Theorem~\ref{thm:strong.equivalence}}
For the ``if'' direction, the result is straightforward: when $\models \alpha \leftrightarrow \beta$, $\alpha$ and $\beta$ have the same models, and so, also $\Delta \cup \{\alpha\}$ and $\Delta \cup \{\beta\}$  have the same models, for any theory $\Delta$, so they also have the same equilibrium models.
For the ``only if'' direction we will proceed by contraposition, i.e., we will prove that $\not\models \alpha \leftrightarrow \beta$ implies that $\alpha$ and $\beta$ are not strongly equivalent.
If $\not\models \alpha \leftrightarrow \beta$ there is some model $\tuple{H,T}$ of one of the formulas that is not model of the other. Without loss of generality, suppose $\tuple{H,T} \models \alpha$ and $\tuple{H,T} \not\models \beta$.
Then, by Lemma~\ref{lem:strong.equivalence.aux}, $\alpha$ and $\beta$ are not strongly equivalent.
\end{proofof}

%%%%%%%%%%%%%%%%%%%%%%%%%%%%%%%%%%%%%%%%
\begin{proofof}{Theorem~\ref{th:substeq}}
For the ``if'' direction, if $\models \alpha \Leftrightarrow \beta$ we conclude $\models \varphi[\alpha/p] \Leftrightarrow \varphi[\beta/p]$ by Theorem~\ref{th:subst}.
But then, $\varphi[\alpha/p]$ and $\varphi[\beta/p]$ share the same models, and thus, $\Delta \cup \{\varphi[\alpha/p]\}$ and $\Delta \cup \{\varphi[\alpha/p]\}$ also have the same models for any $\Delta$, so they also share the same equilibrium models.
For the ``only if'' direction, note that if $\alpha$ and $\beta$ are strongly equivalent on substitutions, they are also strongly equivalent and, from Theorem~\ref{thm:strong.equivalence}, this implies that $\models \alpha \leftrightarrow \beta$.
Furthermore,
if $\alpha$ and $\beta$ are strongly equivalent on substitutions,
we also get that
$\sneg\alpha$ and $\sneg\beta$ are strongly equivalent.
From Theorem~\ref{thm:strong.equivalence}, this implies that $\models \sneg\alpha \leftrightarrow \,\sneg\beta$.
Hence,
we obtain that
$\models \alpha \Leftrightarrow \beta$.
\end{proofof}
